# Supplementary material for: RECIPE4U: Student-ChatGPT Interaction Dataset in EFL Writing Education
Source: arXiv:2403.08272 source file (2024-03-13)
Supplement: Supplementary file 1 [file appendix.tex]

\section{Experimental Setting}
\label{sec:experimental_setting}

\subsection{Hyperparameters for Fine-tuning Models}

Table \ref{tab:model_config} shows hyperparameter settings of our models.
We used Intel(R) Xeon(R) Silver 4114 (40 CPU cores) and GeForce RTX 2080 Ti 10GB (4 GPUs) for all experiments using M-BERT~\cite{devlin-etal-2019-bert} and XLM-R~\cite{conneau-etal-2020-unsupervised}.
\begin{table}[!h]
\centering
\begin{tabular}{@{}ll@{}}
\toprule
Hyperparameter          & Value  \\ \midrule
Batch Size              & 32     \\
Early Stopping Patience & 3      \\
Hidden Size             & 768    \\
Learning Rate           & 2e-5   \\
Learning Rate Scheduler & Linear \\
Max Sequence Length     & 512    \\
Number of Hidden Layers & 12     \\
Optimizer               & AdamW  \\ \bottomrule
\end{tabular}
\vspace{-3mm}
\caption{Model configuration}
\label{tab:model_config}
\end{table}

\subsection{Prompts for Intent Detection Model Inferences}

\noindent\fbox{%
    \parbox{\columnwidth}{%
        <Prompt 1>
        The following sentence is an utterance of a student taking an EFL writing class during a conversation with AI.
        Read the sentence and choose one intention from 13 labels. Answer in two list formats: div1, div2.\\
        \texttt{\$Label Explanation}\\
        \texttt{\$Label Examples}
}}

\noindent\fbox{%
    \parbox{\columnwidth}{%
        <Prompt 2>
        The following sentence is an utterance by a student participating in an EFL writing class while talking to AI. Carefully read the sentence, choose all the intentions from \$labels, and answer in two list formats: div1, div2.\\
        \texttt{\$Label Explanation}\\
        \texttt{\$Label Examples}
}}

\noindent\fbox{%
    \parbox{\columnwidth}{%
        <Prompt 3>
        The sentence below is an utterance by a student taking an EFL writing class during a conversation with AI. Read the sentence, find all the intentions from \$labels, and make two lists: div1, div2.\\
        \texttt{\$Label Explanation}\\
        \texttt{\$Label Examples}
}}

\noindent\fbox{%
    \parbox{\columnwidth}{%
        <Prompt 4>
        The following is an utterance from a student during a conversation between a student taking an EFL writing class and AI. Read the sentence and choose all the intentions from \$labels, then answer in two list formats: div1, div2.\\
        \texttt{\$Label Explanation}\\
        \texttt{\$Label Examples}
}}

\noindent\fbox{%
    \parbox{\columnwidth}{%
        <Prompt 5>
        This sentence is an utterance by a student taking an EFL writing class during a conversation with AI. Analyze the sentence and choose all the intentions from \$labels in div1 and div2 respectively.\\
        \texttt{\$Label Explanation}\\
        \texttt{\$Label Examples}
}}

\subsection{Prompts for Satisfaction Estimation Model Inferences}

\noindent\fbox{%
    \parbox{\columnwidth}{%
        <Prompt 1>
        The following utterences are dialogue turn of a student taking an EFL writing class and AI. Read two sentences and rate the helpfulness of response from AI to students in 5 Likert scale as the EFL writing class student. Answer only with one number.\\
        \texttt{\$Satisfaction Examples}
}}

\noindent\fbox{%
    \parbox{\columnwidth}{%
        <Prompt 2>
        The following is a conversation of a student taking an EFL writing class and AI. You are the student and rate the helpfulness of the utterance of AI in 1-5 scale. Answer one number only\\
        \texttt{\$Satisfaction Examples}
}}

\noindent\fbox{%
    \parbox{\columnwidth}{%
        <Prompt 3>
        The following sentences are a turn in conversation between EFL writing class student and AI. Act as the student and score the helpfulness of the utterance of AI in 5 Likert scale. You should answer only in one number\\
        \texttt{\$Satisfaction Examples}
}}

\noindent\fbox{%
    \parbox{\columnwidth}{%
        <Prompt 4>
        The following is a part of conversation between student participating an EFL writing class and AI. Assume you are that student and rate the helpfulness of AI response in 1-5 score. Please answer only in one number\\
        \texttt{\$Satisfaction Examples}
}}

\noindent\fbox{%
    \parbox{\columnwidth}{%
        <Prompt 5>
        The sentences are a dialogue turn in conversation between EFL writing class student and AI. You are the student taking an EFL writing class and rate AI response helpfulness in 1-5 numbers. Answer with only one number\\
        \texttt{\$Satisfaction Examples}
}}

% \clearpage

\section{Student Dialogue Intent Labels}

Table~\ref{tab:intent_label} shows the labels of intent for student dialogue.
